# Supplementary material for: SAGA: A Participant-specific Examination of Story Alternatives and Goal Applicability for a Deeper Understanding of Complex Events
Source: arXiv:2408.05793 source file (2024-08-11)
Supplement: Supplementary file 1 [file appendix_results.tex]

\subsubsection{Additional Results for Goal Inference }
\label{app:task1-additional-results}

\begin{table*}[t]
\centering
\resizebox{.98\textwidth}{!}{
 \begin{tabular}{l|l|c|c|c|c|c|c|c|c|c|c|c|c|}
 \cline{2-14}
  &  & \multicolumn{3}{|c|}{Rouge} & MET- & \multicolumn{2}{|c|}{BLEU} & Bert-&\multicolumn{5}{|c|}{Human Evaluation}\\ 
  & & R1 & R2 & RL & EOR & Corpus & Google & Score&Cohere &Explain & Faith & Truth & Intent\\
 \cline{2-14}
 \cline{2-14}
 &Reference & \multicolumn{7}{|c|}{-} &4.76 & 4.67 & 4.9 & 4.91 & 4.74 \\ 
 \cline{2-14}
\multirow{6}{*}{Val Split} 
& T5-11b  &  &  &  &  &  &  & &&&&& \\
& flanT5b  &  .37  &  .14 & .36 & .34  &  0.9 & .14 &.86& 3.72- & 3.94- &4.15-&3.79- & 3.64-  \\
& flanT5l  & .41  & .22  & .4 & .3  & .16  & .14 & .84 &&&&&\\
& flanT5xl & .42  & .21 & .4 & .33  & .17  & .15 & .85&&&&&\\
& flanT5xxl&  .45 & .25 & .44 & .43  & .2  & .2 & .86 &4.5&4.37&4.86&4.92 &4.38\\
& gpt3.5t  &  .44 & .21 & .42 &  .49 & .11  & .15 & &4.68&\textbf{4.93+}&4.86&4.86&4.42\\
& gpt4     & .5  & .3 & .49 &.51   &.21   & .23 & &4.94&4.9&4.98&4.98&4.86\\
\hline
\multirow{10}{*}{Act.}&\multirow{5}{*}{Val}
 &\multicolumn{3}{|l|}{Ref mean vals (var < \%) }&4.81&4.78 &4.91 &4.97 &4.82 \\ 
&& Ref    &&      &4.73 &4.76 &4.96 &5.00 &4.84 \\
&&fT5b    &.38&.36&\underline{3.61}&\underline{3.85}&\underline{4.20}&\underline{3.69}&\underline{3.52} \\ 
&& Ref    &&      &4.83 &4.79 &4.84 &4.92 &4.75 \\
&& fT5xxl &.44&.44&4.47 &4.43 &4.93 &4.92 &4.37 \\
&& Ref    &&      &4.75 &4.68 &4.87 &5.00 &4.69 \\
&& gpt3.5t&.43&.50&4.67 &\textbf{4.96}&4.84 &4.84 &4.53 \\
&& Ref    &&      &4.92 &4.88 &4.96 &4.96 &4.83 \\
&& gpt4   &.48&.53&4.91 &4.87 &5.00 &5.00 &4.8\\
\cline{2-10}
&\multirow{5}{*}{Test} 
 &\multicolumn{3}{|l|}{Ref mean vals (var < \%) }&4.74&4.69&4.78&4.78&4.49 \\ 
&& Ref    &&      &4.73 &4.67 &4.78 &4.85 &4.43 \\
&& fT5b   &.42&.40&\underline{3.95}&\underline{4.19}&4.50 &\underline{4.35}&\underline{3.72} \\
&& Ref    &&      &4.75 &4.71 &4.77 &4.88 &4.54 \\
&& fT5xxl &.50&.49&4.49 &4.65 &4.83 &4.81 &\underline{4.03} \\
&& Ref    &&      &4.73 &4.65 &4.76 &4.74 &4.49 \\
&& gpt3.5t&.44&.52&4.53 &4.59 &\textbf{4.95}&\underline{3.89}&4.90 \\
&& Ref    &&      &4.75 &4.71 &4.81 &4.81 &4.48 \\
&& gpt4   &.53&.55&\underline{4.46}&4.44 &4.82 &4.82 &\underline{3.92}\\
\hline
\hline
  &Reference & \multicolumn{7}{|c|}{-} &4.74 & 4.73 & 4.79 & 4.83 & 4.57 \\ 
\hline
\multirow{6}{*}{Test Split} 
& T5-11b  &  &  &  &  &  &  & &&&&& \\
& flanT5b & .44 & .21 & .42 & .4 & .11 & .16 & .86 &3.47-&3.78-&4.1-&3.97-&3.32-\\
& flanT5l &.45 & .23 & .45 & .32 & .18 & .15 & .86 &&&&&\\
& flanT5xl  & .47 & .25 & .46 & .36  & .18 & .16 & .86 &&&&&\\
& flanT5xxl  & .50 & .27  & .49 & .46  & .2  & .2 & .86&4.31-&4.47- &4.67&4.71&4.0-\\
& GPT3.5t & .44 & .22 & .42 &  .49&  .1 & .14&&4.47-&4.47-&4.86&4.81&3.9-\\
& GPT4  & .52 & .32 & .51 & .53 & .22 & .24 &  &4.53&4.49&4.81&4.82&4.00-\\
 \hline
 \cline{2-9}
 \end{tabular}
 }
 \caption{Automated and Human Evaluation scores for model generated Goals. }
\label{tab:goal-description-all-metrics}
\end{table*}

\subsubsection{Additional Results for Explainable Next Action Inference}
\label{app:task2-additional-results}

\begin{table}[t]
 \centering
\resizebox{.98\columnwidth}{!}{
 \begin{tabular}{|l|c|c|c|c|c|c|c|c|}
 \hline
& \multicolumn{4}{|c|}{Val} & \multicolumn{4}{|c|}{Test}\\ 
& \multicolumn{2}{|c|}{Action} & \multicolumn{2}{|c|}{Explanation}&\multicolumn{2}{|c|}{Action} & \multicolumn{2}{|c|}{Explanation}\\ 
%Split&
Model&Acc&mF1&Acc&mF1&Acc&mF1&Acc&mF1\\
\hline
%\multirow{5}{*}{Val} 
 Maj.   &.77&.29&.79&.44 &.66&.27&.70&.41\\ 
 T511b  &.64&.32&.58&.49 &.56&.31&.50&.47\\
 fT5b   &.76&.36&.74&.59 &.64&.30&.70&.63\\
 fT5l   &.75&.40&.80&.69 &.62&.37&.78&.74 \\
 fT5xl  &.81&.49&.72&.67 &.68&.43&.71&.70\\
 fT5xxl &.78&.49&.79&.73 &.68&.45&.78&.76 \\
 gpt3.5t&.39&.30&.60&.54 &.46&.37&.57&.54\\
 gpt4   &\textbf{.82}&\textbf{.50}&\textbf{.86}&.\textbf{76} &\textbf{.75}&\textbf{.47}&\textbf{.84}&\textbf{.80}\\
 \hline
 T5b-ft &&&.64&.56 &&&.66&.61\\
 fT5b-ft&&&.75&.66&&&.70&.64 \\
\hline
\end{tabular}
}
 \caption{Next Action Transferability }
\label{tab:all-next-action-transfer-metrics}
\end{table}
Next action applicability inference task identifies if a next action obtained for $S^a$ or $S^c_k$ is Most Likely, Somewhat Likely or Unlikely for a given $(S^{c_k},P_{ij})$.  We cast identifying Explanation transferability as a binary inference where explanations obtained for $S^a$'s next actions can explain $S^c_k$'s next actions.

\subsubsection{Additional Results for  Goal Achievement Plan Inference}
\label{app:task4-additional-results}

1) what is the difference between few-shot \& fine tuned
2)difference between large and small in fewshot \& fine tuned?
3)
\begin{table}[t]
 \centering
\resizebox{.98\columnwidth}{!}{
 \begin{tabular}{|l|c|c|c|c|c|c|c|c|c|c|}
 \hline
 & \multicolumn{5}{|c|}{Actual Story} & \multicolumn{5}{|c|}{Counterfactual Story}\\  Model  & Rou  & ME&P. Type&\multicolumn{2}{|c|}{Human Eval.} & Rou &ME&P. Type&\multicolumn{2}{|c|}{Human Eval.}\\ 
  Type&  L &TR &Acc/F1& Plan &Type&  L &TR&Acc/F1& Plan &Type\\
 \hline
\hline
Maj.     &&&.62/.77&     & &&&.62/.77&&\\
Ref    &&&&4.28&4.28& &&&4.31&4.29 \\ 
%&&Ref    &&&&&4.25&3.95 &&&&&4.34&4.34\\
fT5b &.19&.24&.59/.74 &\underline{3.15} & \underline{2.49} &.20&.24&.63/.77&\underline{3.31}& \underline{2.32}\\
%&&Ref    &&&&&4.20&4.20 &&&&&4.23&4.23\\
fT5xxl &.22&.24&.62/.77&4.10&\underline{2.14}&.17&.20&.62/.77&3.57&\underline{2.12}\\
%&&Ref    &&&&4.29&4.29&  &&&&&4.39&4.36\\
gpt3.5t&.19&.28&.62/.77&4.07&\underline{2.41}&.17&.26&.62/.76&3.92&\underline{2.51}\\
%&&Ref    &&&&&4.29&4.23 &&&&&4.37&4.37 \\
gpt4  &.19&.29&.62/.77&4.36&\underline{2.34}&.18&.29&.62/.77&4.07&\underline{2.78}\\
\hline
%T5b-ft  &.38&.37&.68/.81&-&-&.39&.37&.82/.90&-&- \\ #without unachievable in test
T5b-ft  &.36&.34&.58/.74&-&-&.36&.31&.58/.73&-&- \\ %.16,.11,.70/.78,.12,.10,.77/.83 (epoch 5)
%with unachievable in training T5b-ft  &.40&.36&.55/.66&-&-&.44&.38&.50/.45&-&- %epoch2 for actual and epoch 4 for counterfactual\\
fT5b-ft&.40&.36&.58/.74&-&-&.36&.30&.58/.73&-&-\\ 
%.16,.10,.72/.79,.12,.09,  .87/.90
%fT5b-ft&.42&.39&.43/.17&-&-&.40&.36&.82/.90&-&-\\ 
fT5l-ft&.38&.35&.58/.74&-&-&.36&.31&.58/.73&-&-\\
%.16,.12,.78/.82,.15,.11,.86/.89
\hline
\end{tabular}
}
 \caption{Evaluation of model generated plans and plan types (revised vs. original). }
\label{tab:future-plan-manual-metrics3}
\vspace{-3mm}
\end{table}
\subsubsection{Goal Achievement \& Satisfaction Inference}
\label{app:task5-additional-results}

\begin{table*}[t]
 \centering
\resizebox{.98\textwidth}{!}{
 \begin{tabular}{l|l|c|c|c|c|c|c|c|c|c|c|c|c|}
 \cline{2-13}
  &  & \multicolumn{3}{|c|}{Rouge} & MET- & \multicolumn{2}{|c|}{BLEU} & Bert-&\multicolumn{4}{|c|}{Human Evaluation}\\ 
  & & R1 & R2 & RL & EOR & Corpus & Google & Score&Cohere &Cohesive & Explain & Correct\\
 \hline
  
\hline
\multirow{6}{*}{Val Split} 
 &Reference & \multicolumn{7}{|c|}{-} &4.65 & 4.60 & 4.79 &  - \\
 \hline
 & T5-11b  &  &  &  &  &  &  & &&&&\\
& flanT5b  &  .32  &  .19 & .3 & .3  &  0.19 & .19 &.85& 1.9- & 1.71- & 1.3- &1.23-  \\
& flanT5l  & .16  & .05  & .15 & .12  & .03  & .07 & .84 &&&&\\
& flanT5xl & .25  & .16 & .23 & .22  & .12  & .15 & .85&&&&\\
& flanT5xxl&  .48 & .36 & .45 & .49  & .34  & .32 & .86 &4.78&4.47&4.2-&4.73 \\
& gpt3.5t  &   &  &  &   &   &  & &4.84&4.78&4.88&4.94\\
& gpt4     & .5  & .35 & .46 &.51   &.32   & .31 & &4.9&4.88&4.92&4.88\\
\hline
\hline
  &Reference & \multicolumn{7}{|c|}{-} &4.73 & 4.59 & 4.82 &  - \\ 
\cline{2-13}
\multirow{6}{*}{Test Split} 
& T5-11b  &  &  &  &  &  &  & &&&& \\
& flanT5b & .32 & .2 & .31 & .31 & .2 & .2 & .85 &2.12-&2.08-&1.48-&1.41-\\
& flanT5l &.16 & .05 & .15 & .12 & .02 & .06 & .85 &&&&\\
& flanT5xl  & .26 & .16 & .24 & .23  & .12 & .15 & .86 &&&&\\
& flanT5xxl  & .50 & .37  & .47 & .5  & .35  & .33 & .86&4.29&4.47 &3.83-&4.05-\\
& GPT3.5t &  &  &  &  &  &  &  &4.82&4.66&4.83&4.86\\
& GPT4  & .52 & .32 & .51 & .53 & .22 & .24 &  &4.75&4.66&4.91&4.99\\
 \hline
 \cline{2-9}
 \end{tabular}
 }
 \caption{Automated and Human Evaluation scores for model generated Next Actions. }
\label{tab:next-action-automated-metrics}
\end{table*}

\begin{table}[t]
 \centering
\resizebox{.98\columnwidth}{!}{
 \begin{tabular}{|l||l|l|c|c|c|c|c|c|}
 \hline
  Story &Split&Model  & Rouge & MET &\multicolumn{2}{|c|}{Plan Type}&\multicolumn{2}{|c|}{Human Eval.}\\ 
  Type& & & L & EOR &Acc&F1& Plan &Rev\\
 \hline
\hline
\multirow{10}{*}{Act.}&\multirow{6}{*}{Val.}&
Maj      &&&.79&.44&& \\ 
&&Ref    &&&&&4.23&4.23 \\
%&&Ref    &&&&&4.17&4.17 \\
&&fT5b   &.19&.20&.79&.44& 3.43 & \underline{2.67}\\
%&&Ref    &&&&3.95&3.95& \\
&&fT5xxl &.19&.22&.79&.44&4.14&\underline{2.79}\\
%&&Ref    &&&&&4.57&4.57 \\
&&gpt3.5t&.19&.29&.79&.44&4.5&\underline{2.14}\\
%&&Ref    &&&&&4.24&4.24 \\
&&gpt4   &.20&.31&.79&.44&3.86&\underline{1.48}\\
\cline{2-9}
&\multirow{5}{*}{Test}&
Maj.     &&&.62&.38&&\\
&&Ref    &&&&&4.28&4.28 \\ 
%&&Ref    &&&&&4.25&3.95 \\
 && fT5b &.19&.24&.79&.47 &\underline{3.18} & \underline{2.42}\\
%&&Ref    &&&&&4.20&4.20 \\
&&fT5xxl &.22&.24&.62&.38&4.23&\underline{2.98}\\
%&&Ref    &&&&4.29&4.29& \\
&&gpt3.5t&.19&.28&.62&.38&4.16&\underline{2.60}\\
%&&Ref    &&&&&4.37&4.37 \\
&& gpt4  &.19&.29&.62&.38&4.36&\underline{2.63}\\
\hline
\hline
\multirow{10}{*}{Cou.}&\multirow{5}{*}{Val}&
Maj      &&&.80&.45&& \\ 
&&Ref & &&&&4.11&4.12 \\ 
%&&Ref    &&&&&4.31&4.21 \\
&& fT5b   &.17&.20&.59&.42& \underline{3.15} & \underline{2.93}\\
%&&Ref    &&&&&4.19&4.09 \\
&& fT5xxl &.17&.20&.80&.45&\textbf{4.72}&\underline{2.80}\\
%&&Ref    &&&&&4.24&4.15 \\
&& gpt3.5t&.16&.25&.80&.45&4.5&\underline{2.09}\\
%&&Ref    &&&&&4.12&4.03 \\
&& gpt4  &.17&.27&.78&.44&4.2&\underline{1.59}\\
\cline{2-9}
&\multirow{5}{*}{Test} &
Maj      &&&.62&.38&& \\ 
&&Ref & &&&&4.31&4.29 \\ 
%&&Ref    &&&&&4.34&4.34 \\
&& fT5b   &.20&.24&.63&.40&\underline{3.31}& \underline{2.70}\\
%&&Ref    &&&&&4.23&4.23 \\
&& fT5xxl &.20&.23&.62&.38&3.80&\underline{2.87}\\
%&&Ref    &&&&&4.39&4.36 \\
&& gpt3.5t&.17&.26&.62&.38&4.04&\underline{2.44}\\
%&&Ref    &&&&&4.29&4.23 \\
&& gpt4   &1.8&.29&.62&.38&4.16&\underline{2.11}\\
\hline
\end{tabular}
}
 \caption{Automated and Human Evaluation scores for model generated Plans for goal achievement. }
\label{tab:future-plan-manual-metrics2}
\end{table}

\emph{\textbf{Are larger models better at identifying goal achievement within a Story and After?}}
We first examine if a selected participant's goal is achieved within the story formulating it as an entailment task with either ($S^a$, $G_ij$) or ($S^c_k$,$G_ij$) as the premise and asking whether $P_i$ achieved the goal by the end of the story with the options of Yes, No and Unsure.  Since next actions are logically continuous with the story we extend this entailment to include the next action in the premise. While larger models are better with the exception of T511b, 
%(see \cref{tab:goals-success-in-story-metrics} and \cref{tab:all-goals-success-in-story-metrics} for additional models) 
fine-tuning leads to similar performance for all model sizes.

\begin{table}[t]
 \centering
\resizebox{.98\columnwidth}{!}{
 \begin{tabular}{|l|l|c|c|c|c|}
 \hline
&& \multicolumn{2}{|c|}{Actual} & \multicolumn{2}{|c|}{Counterf.}\\ 
Split&Model&Acc&mF1&Acc&mF1\\
\hline
\multirow{5}{*}{Val} 
& Maj.    &.69&.27&.72&.28 \\ 
& T511b   &.59&.39&.48&.32 \\
& T5b-ft  &.82&.54&.53&.36 \\
& fT5b    &.67&.30&.70&.37 \\
& fT5b-ft &.78&.51&.46&.30 \\
& fT5l    &.84&.55&.61&.38 \\
& fT5l-ft &.84&.55&.61&.38 \\
& fT5xl   &.91&.62&.58&.37 \\
& fT5xl-ft&.91&.62&.58&.37 \\
& fT5xxl  &.93&.63&.60&.38 \\
& gpt3.5t &.89&.71&.66&.46 \\
& gpt4    &.89&.60&.59&.37 \\
 \hline
\hline
\multirow{5}{*}{Test} 
& Maj.    &.71&.28&.68&.27 \\ 
& T511b   &.53&.33&.48&.31 \\
& T5b-ft  &.79&.52&.51&.34 \\
& fT5b    &.78&.45&.63&.35 \\
& fT5b-ft &.80&.54&.47&.32 \\
& fT5l    &.78&.51&.56&.37 \\
& fT5l-ft &.78&.51&.56&.37 \\
& fT5xl   &.88&.58&.51&.35- \\
& fT5xl-ft&.88&.58&.51&.35- \\
& fT5xxl  &.87&.58&.57&.37 \\
& gpt3.5t &.90&.60&.58&.38 \\
& gpt4    &.90&.60&.57&.38 \\
\hline
\end{tabular}
}
 \caption{Model identification of Goal achievement direction after the story end.  }
\label{tab:all-goals-direction-after-story-metrics}
\end{table}

\begin{table}[t]
 \centering
\resizebox{.98\columnwidth}{!}{
 \begin{tabular}{|l|l|c|c|c|c|}
 \hline
&& \multicolumn{2}{|c|}{Actual} & \multicolumn{2}{|c|}{Counterf.}\\ 
Split&Model&Acc&mF1&Acc&mF1\\
\hline
\multirow{5}{*}{Val} 
& Maj.   &.74&.28&.69&.27 \\ 
& T511b  &.62&.34&.56&.31 \\
& fT5b   &.80&.45&.68&.36 \\
& fT5l   &.83&.54&.64&.43 \\
& fT5xl  &.83&.53&.61&.43 \\
& fT5xxl &.86&.56&.71&.47 \\
& gpt3.5t&.84&.54&.69&.47 \\
& gpt4   &.84&.54&.72&.48 \\
 \hline
\hline
\multirow{5}{*}{Test} 
& Maj.   &.72&.28&.62&.26 \\ 
& T511b  &.60&.33&.52&.32 \\
& fT5b   &.74&.36&.64&.36 \\
& fT5l   &.75&.48&.58&.40 \\
& fT5xl  &.70&.47&.67&.46 \\
& fT5xxl &.87&.58&.66&.45 \\
& gpt3.5t&.84&.54&.63&.48 \\
& gpt4   &.87&.57&.67&.50 \\
\hline
\end{tabular}
}
\caption{Participant's satisfaction with the state of goal achievement}
\label{tab:goal-satisfaction-metrics}
\end{table}

\begin{table*}[t]
 \centering
 \begin{tabular}{|l|l|c|c|c|c|c|c|}
 \hline
Story Type& Model & \multicolumn{3}{|c|}{Rouge} & Met & \multicolumn{2}{|c|}{BLEU} \\ 
(split)  & & R1 & R2 & RL & eor & Cor. & Sen. \\ 
\hline
\hline
\multirow{3}{*}{Actual Stories} 
& T5-11b (3-shot) & .15 & .07 & .14 &  .26& .03 & .03 \\
\multirow{3}{*}{\textbf{(Val.) }} 
 & flanT5b (3-shot)  & .39 & .16  & .38 &  .36 & .09  & .14 \\
& flanT5l (3-shot)  &  .43 &  .24 & .42 &  .31 &  .18 & .15 \\
& flanT5xl (3-shot) &  .44 & .23 & .43 & .35  &  .18 & .16 \\
& flanT5xxl(3-shot) &  .45 & .26 & .44 & .44  & .20  & .19 \\
& gpt3.5t (3-shot)  &  .45 & .26  & .43 & .50  & .14  & .17 \\
& gpt4    (3-shot)  & .51  & .30 & .48 &.53   &.20   & .23\\
\hline
\multirow{3}{*}{Alternative Stories} 
& T5-11b (3-shot)  & .15 & .06 & .13 & .26 & .02 & .03 \\
\multirow{3}{*}{\textbf{(Val.)}} 
 & flanT5b (3-shot)  &  .35  & .11 &  .34&  .31 & .97 & .12 \\
& flanT5l  (3-shot) &  .36  &  .16 & .35 & .26  & .12  & .11 \\
& flanT5xl (3-shot) &   .41 & .19 & .38  & .31  &  .15 & .14  \\
& flanT5xxl(3-shot) &  .44 & .23 & .42 & .41  & .17  & .17 \\
& gpt3.5t (3-shot)  &  .42 & .22 & .40 & .46  &  .12 & .15 \\
& GPT4  (3-shot) & .47 & .27 & .46 & .49 & .21 & .23 \\

\hline
\hline
\multirow{3}{*}{Actual Stories} 
& T5-11b  & .16 & .06 & .14 & .28 & .02 & .03\\
\multirow{3}{*}{\textbf{(Test)}} 
& flanT5b (3-shot) &  .43 & .21 &  .42 & .40  & .12  & .16 \\
& flanT5l (3-shot) & .45 & .24  & .45 & .33  & .18  & .15  \\
& flanT5xl (3-shot)  & .48 &  .25 & .46  & .36  & .17  & .15 \\
& flanT5xxl  (3-shot) & .52 & .29  & .50 & .49  & .21  & .22 \\
& GPT3.5t(3-shot)  &  .45  & .25 & .44 &.52   &.13   & .17 \\
& gpt4     (3-shot) & .55  & .33 & .54 &.55   &.23   & .26 \\
\hline
\multirow{3}{*}{Alternative Stories} 
& T5-11b (3-shot)  & .16 & .06 & .14 & .26 & .02 & .03 \\
\multirow{3}{*}{\textbf{(Test)}} 
& flanT5b (3-shot) &  .43 & .19 & .42  & .39  & .10  & .15  \\
& flanT5l (3-shot) & .44 & .20 & .43  & .31  & .16  & .14   \\
& flanT5xl  (3-shot) &  .44 & .22  & .43  &  .33  & .17  & .15   \\
& flanT5xxl  (3-shot) & .47 & .26  & .46 & .44  & .18  & .19 \\
& GPT3.5t (3-shot) &  .43&  .23& .42 & .48 & .11 & .15 \\
& GPT4  (3-shot) & .49 & .28 & .48 & .49 & .19 & .22 \\
 \hline
 \hline
 \end{tabular}
 \caption{Automated Evaluation scores for model generated goals.  BertScore value was .86 for all models and story types.%\todo[inline]{fix table}
 }
\label{tab:goal-automated-metrics}
\end{table*}
